# Supplementary material for: A Tutorial on 5G Positioning
Source: arXiv:2311.10551 source file (2024-09-12)
Supplement: Supplementary file 1 [file appendix.tex]

\appendix
\label{apx:crb}
\setcounter{equation}{0}

%\subsection*%{Demonstration of Cram\'{e}r-Rao Bound}%
%\mb{ADD REFs}
% \textcolor{blue}{The \ac{CRB} is a well-known lower bound in the localization field. In general, the \ac{CRB} sets the lower value of the covariance for any unbiased estimator with parametric \ac{PDF}. This minimum value can be asymptotically approached by the maximum likelihood estimator when dealing with a large number of observations. While the explicit form of the estimator may not always be available, the \ac{CRB} can consistently be computed in a closed form \cite{spagnolini18}.}
%\subsubsection{Proof}

\textcolor{blue}{Let $\boldsymbol{\hat{u}}$ be the unbiased estimator for the \ac{UE} true position $\boldsymbol{u}$ and $\text{ln}\, p(\boldsymbol{\rho} | \boldsymbol{u})$ be the log-likelihood function whose statistics depend on the measurement noise distribution.
The \ac{CRB} sets the bound of the covariance as follows:
\begin{align}
     \text{cov}(\boldsymbol{\hat{u}})
     = \mathbb{E} \left[ (\boldsymbol{\hat{u}}- \boldsymbol{u}) (\boldsymbol{\hat{u}}- \boldsymbol{u})^{\T} \right]
     \geq \boldsymbol{C} (\boldsymbol{u})_{\text{CRB}} = \boldsymbol{J}^{-1}(\boldsymbol{u}).
\end{align}
% The \ac{FIM} $\boldsymbol{J} \in \mathbb{R}^{D\times D}$ has $D$  dimension (e.g., $D=3$ for \ac{3D} scenarios) and its entries are written as:
% \begin{align}
%     \left[ \boldsymbol{J}(\boldsymbol{u}) \right]_{i,j} 
%     &=
%     - \mathbb{E} \left[ \frac{\partial^2 \text{ln}\, p(\boldsymbol{\rho} | \boldsymbol{u})}{ \partial u_i \,\,  \partial u_j} \right]%_{\boldsymbol{u} = \boldsymbol{u}_0}   
%     \nonumber \\
%     &=
%     \mathbb{E} \left[ \frac{ \partial \text{ln}\, p(\boldsymbol{\rho} | \boldsymbol{u})}{ \partial u_i} \frac{ \partial \text{ln} \, p(\boldsymbol{\rho} | \boldsymbol{u})}{ \partial u_j} \right] . %_{\boldsymbol{u} = \boldsymbol{u}_0}. 
% \end{align}
%\mb{Is the denominator correct? It should be bold to me.
\\
The \ac{FIM} $\boldsymbol{J} \in \mathbb{R}^{D\times D}$ has $D$  dimension (e.g., $D=3$ for \ac{3D} scenarios) and it can be written as:
\begin{align}
    \boldsymbol{J}(\boldsymbol{u})  
    = 
    \mathbb{E} \left[ - \frac{\partial^2 \text{ln}\, p(\boldsymbol{\rho} | \boldsymbol{u})}{ \partial \boldsymbol{u} \,\,  \partial \boldsymbol{u}^{\T} } \right]
\end{align}
% with entries of the $i$-th row and $j$-th column calculated as:
% \begin{align}
%     \left[\boldsymbol{J}(\boldsymbol{u})\right]_{i,j}  
%     = 
%     \mathbb{E} \left[ - \frac{\partial^2 \text{ln}\, p(\boldsymbol{\rho} | \boldsymbol{u})}{ \partial \boldsymbol{u}_{i} \,\,  \partial \boldsymbol{u}_{j}^{\T} } \right]
% \end{align}
% }
The demonstration starts from the unbiased condition:
\begin{align}
    \mathbb{E} \left[ \boldsymbol{\hat{u}} - \boldsymbol{u} \right] =  %\left. 
    \int (\boldsymbol{\hat{u}} - \boldsymbol{u}) \, p( \boldsymbol{\rho} | \boldsymbol{u}) \, d \boldsymbol{\rho} % \right|_{\boldsymbol{u} = \boldsymbol{u}_0} 
    = 0.
    \label{eq:app_no_bias}
\end{align}
By applying partial derivative with respect to $\boldsymbol{u}$ on \eqref{eq:app_no_bias}, we obtain the following:
\begin{align}
     &\frac{ \partial}{ \partial \boldsymbol{u}} \left[ %\left. 
     \int (\boldsymbol{\hat{u}} - \boldsymbol{u}) \, p( \boldsymbol{\rho} | \boldsymbol{u}) \, d \boldsymbol{\rho} %\right|_{\boldsymbol{u} = \boldsymbol{u}_0} 
    \right] = 0
 \nonumber \\
     %\left. 
     &\int (\boldsymbol{\hat{u}} - \boldsymbol{u}) \,  p( \boldsymbol{\rho} | \boldsymbol{u}) \frac{ \partial \text{ln} p( \boldsymbol{\rho} | \boldsymbol{u})}{ \partial \boldsymbol{u}} \, d \boldsymbol{\rho} %\right|_{\boldsymbol{u} = \boldsymbol{u}_0} 
    - \boldsymbol{I}_D  \underbrace{\int p( \boldsymbol{\rho} | \boldsymbol{u}) \, d \boldsymbol{\rho} }_1 = 0
\nonumber \\
     %\left. 
     &\int (\boldsymbol{\hat{u}} - \boldsymbol{u}) \,  p( \boldsymbol{\rho} | \boldsymbol{u}) \frac{ \partial \text{ln} p( \boldsymbol{\rho} | \boldsymbol{u})}{ \partial \boldsymbol{u}} \, d \boldsymbol{\rho} %\right|_{\boldsymbol{u} =\boldsymbol{u}_0} 
     = \boldsymbol{I}_D  
%  \\
%       %\left. 
%       \int (\boldsymbol{\hat{u}} - \boldsymbol{u}) \, \frac{ \partial \text{ln} p( \boldsymbol{\rho} | \boldsymbol{u})}{ \partial \boldsymbol{u}} %\right|_{\boldsymbol{u} =\boldsymbol{u}_0} 
%       p( \boldsymbol{\rho} | \boldsymbol{u}_0) \, d \boldsymbol{\rho} &= \boldsymbol{I}_D 
\nonumber \\
      &\mathbb{E} \left[ (\boldsymbol{\hat{u}} - \boldsymbol{u}) \, \frac{ \partial \text{ln} p( \boldsymbol{\rho} | \boldsymbol{u})}{ \partial \boldsymbol{u}} \, d \boldsymbol{\rho} \right]
      %_{\boldsymbol{u} =\boldsymbol{u}_0} 
      = \boldsymbol{I}_D.
      \label{eq:app_unbiased_condition}
\end{align}
%\mb{Missing why we need to consire matrix $\boldsymbol{C} (\boldsymbol{u})$}
}

\textcolor{blue}{
Let us consider the vector 
$
\left[(\boldsymbol{\hat{u}} - \boldsymbol{u}) \,\,  \frac{ \partial \text{ln} p( \boldsymbol{\rho} | \boldsymbol{u})}{ \partial \boldsymbol{u}}\right ]^{\T}
$, 
with covariance
%Using a vector notation, we can define the covariance matrix $\boldsymbol{C} (\boldsymbol{u})$ as:
\begin{align}
    \boldsymbol{C} (\boldsymbol{u}) 
    &=
    \mathbb{E} \left[ \begin{bmatrix} (\boldsymbol{\hat{u}} - \boldsymbol{u}) \\  \frac{ \partial \text{ln} p( \boldsymbol{\rho} | \boldsymbol{u})}{ \partial \boldsymbol{u}}\end{bmatrix} \, \left[ \left(\boldsymbol{\hat{u}} - \boldsymbol{u}\right) \, \left(\frac{ \partial \text{ln} p( \boldsymbol{\rho} | \boldsymbol{u})}{ \partial \boldsymbol{u}}\right) \right]^{\T} \right] 
    \nonumber
    \\
    &=
    \begin{bmatrix}
         \text{cov}(\boldsymbol{\hat{u}}) & \boldsymbol{I}_D \\
        \boldsymbol{I}_D & \boldsymbol{J}(\boldsymbol{u})
    \end{bmatrix},
\end{align}
where the off-diagonal entries are identity matrices thanks to the unbiased property in \eqref{eq:app_unbiased_condition}.
$\boldsymbol{C} (\boldsymbol{u})$ is a block-diagonal matrix,
% Consider the idempotent projection matrix
% \begin{align}
%     \boldsymbol{P} = 
%     \begin{bmatrix}
%         \boldsymbol{I}_D & - \boldsymbol{J}^{-1}(\boldsymbol{u}) \\
%         \boldsymbol{0}_D & \boldsymbol{I}_D 
%     \end{bmatrix}^{\T}
% \end{align}
and, by the properties deriving from the Schur complement, it can be equivalently represented as: 
\begin{align}
   \boldsymbol{C} (\boldsymbol{u})
   &= 
   \begin{bmatrix}
        \boldsymbol{I}_D & - \boldsymbol{J}^{-1}(\boldsymbol{u}) \\
        \boldsymbol{0}_D & \boldsymbol{I}_D 
    \end{bmatrix}
    \begin{bmatrix}
         \text{cov}(\boldsymbol{\hat{u}}) & \boldsymbol{I}_D \\
        \boldsymbol{I}_D & \boldsymbol{J}(\boldsymbol{u}) 
    \end{bmatrix}
    % \begin{bmatrix}
    %     \boldsymbol{I}_D & \boldsymbol{0}_D \\
    %     - \boldsymbol{J}^{-1}(\boldsymbol{u}) & \boldsymbol{I}_D 
    % \end{bmatrix} 
    \begin{bmatrix}
        \boldsymbol{I}_D & - \boldsymbol{J}^{-1}(\boldsymbol{u}) \\
        \boldsymbol{0}_D & \boldsymbol{I}_D 
    \end{bmatrix}^{\T}
    \nonumber
    \\
    &= \begin{bmatrix}
         \text{cov}(\boldsymbol{\hat{u}}) - \boldsymbol{J}^{-1}(\boldsymbol{u}) & \boldsymbol{0}_D \\
        \boldsymbol{0}_D & \boldsymbol{J}(\boldsymbol{u})
    \end{bmatrix}.
\end{align}
Being  $\boldsymbol{C} (\boldsymbol{u})$ a covariance matrix, by definition it is symmetric and positive semi-definite, thus it follows that $ \text{cov}\left(\boldsymbol{\hat{u}}\right) - \boldsymbol{J}^{-1}(\boldsymbol{u}) \geq~0$, demonstrating the lower bound limit of the \ac{CRB}~\cite{spagnolini18}. }
